# Supplementary material for: Robot Skill Adaptation via Soft Actor-Critic Gaussian Mixture Models
Source: arXiv:2111.13129 source file (2022-09-19)
Supplement: Supplementary file 1 [file 7_Appendix.tex]

\begin{figure}[b]
    \centering
    \includegraphics[height=4.5cm]{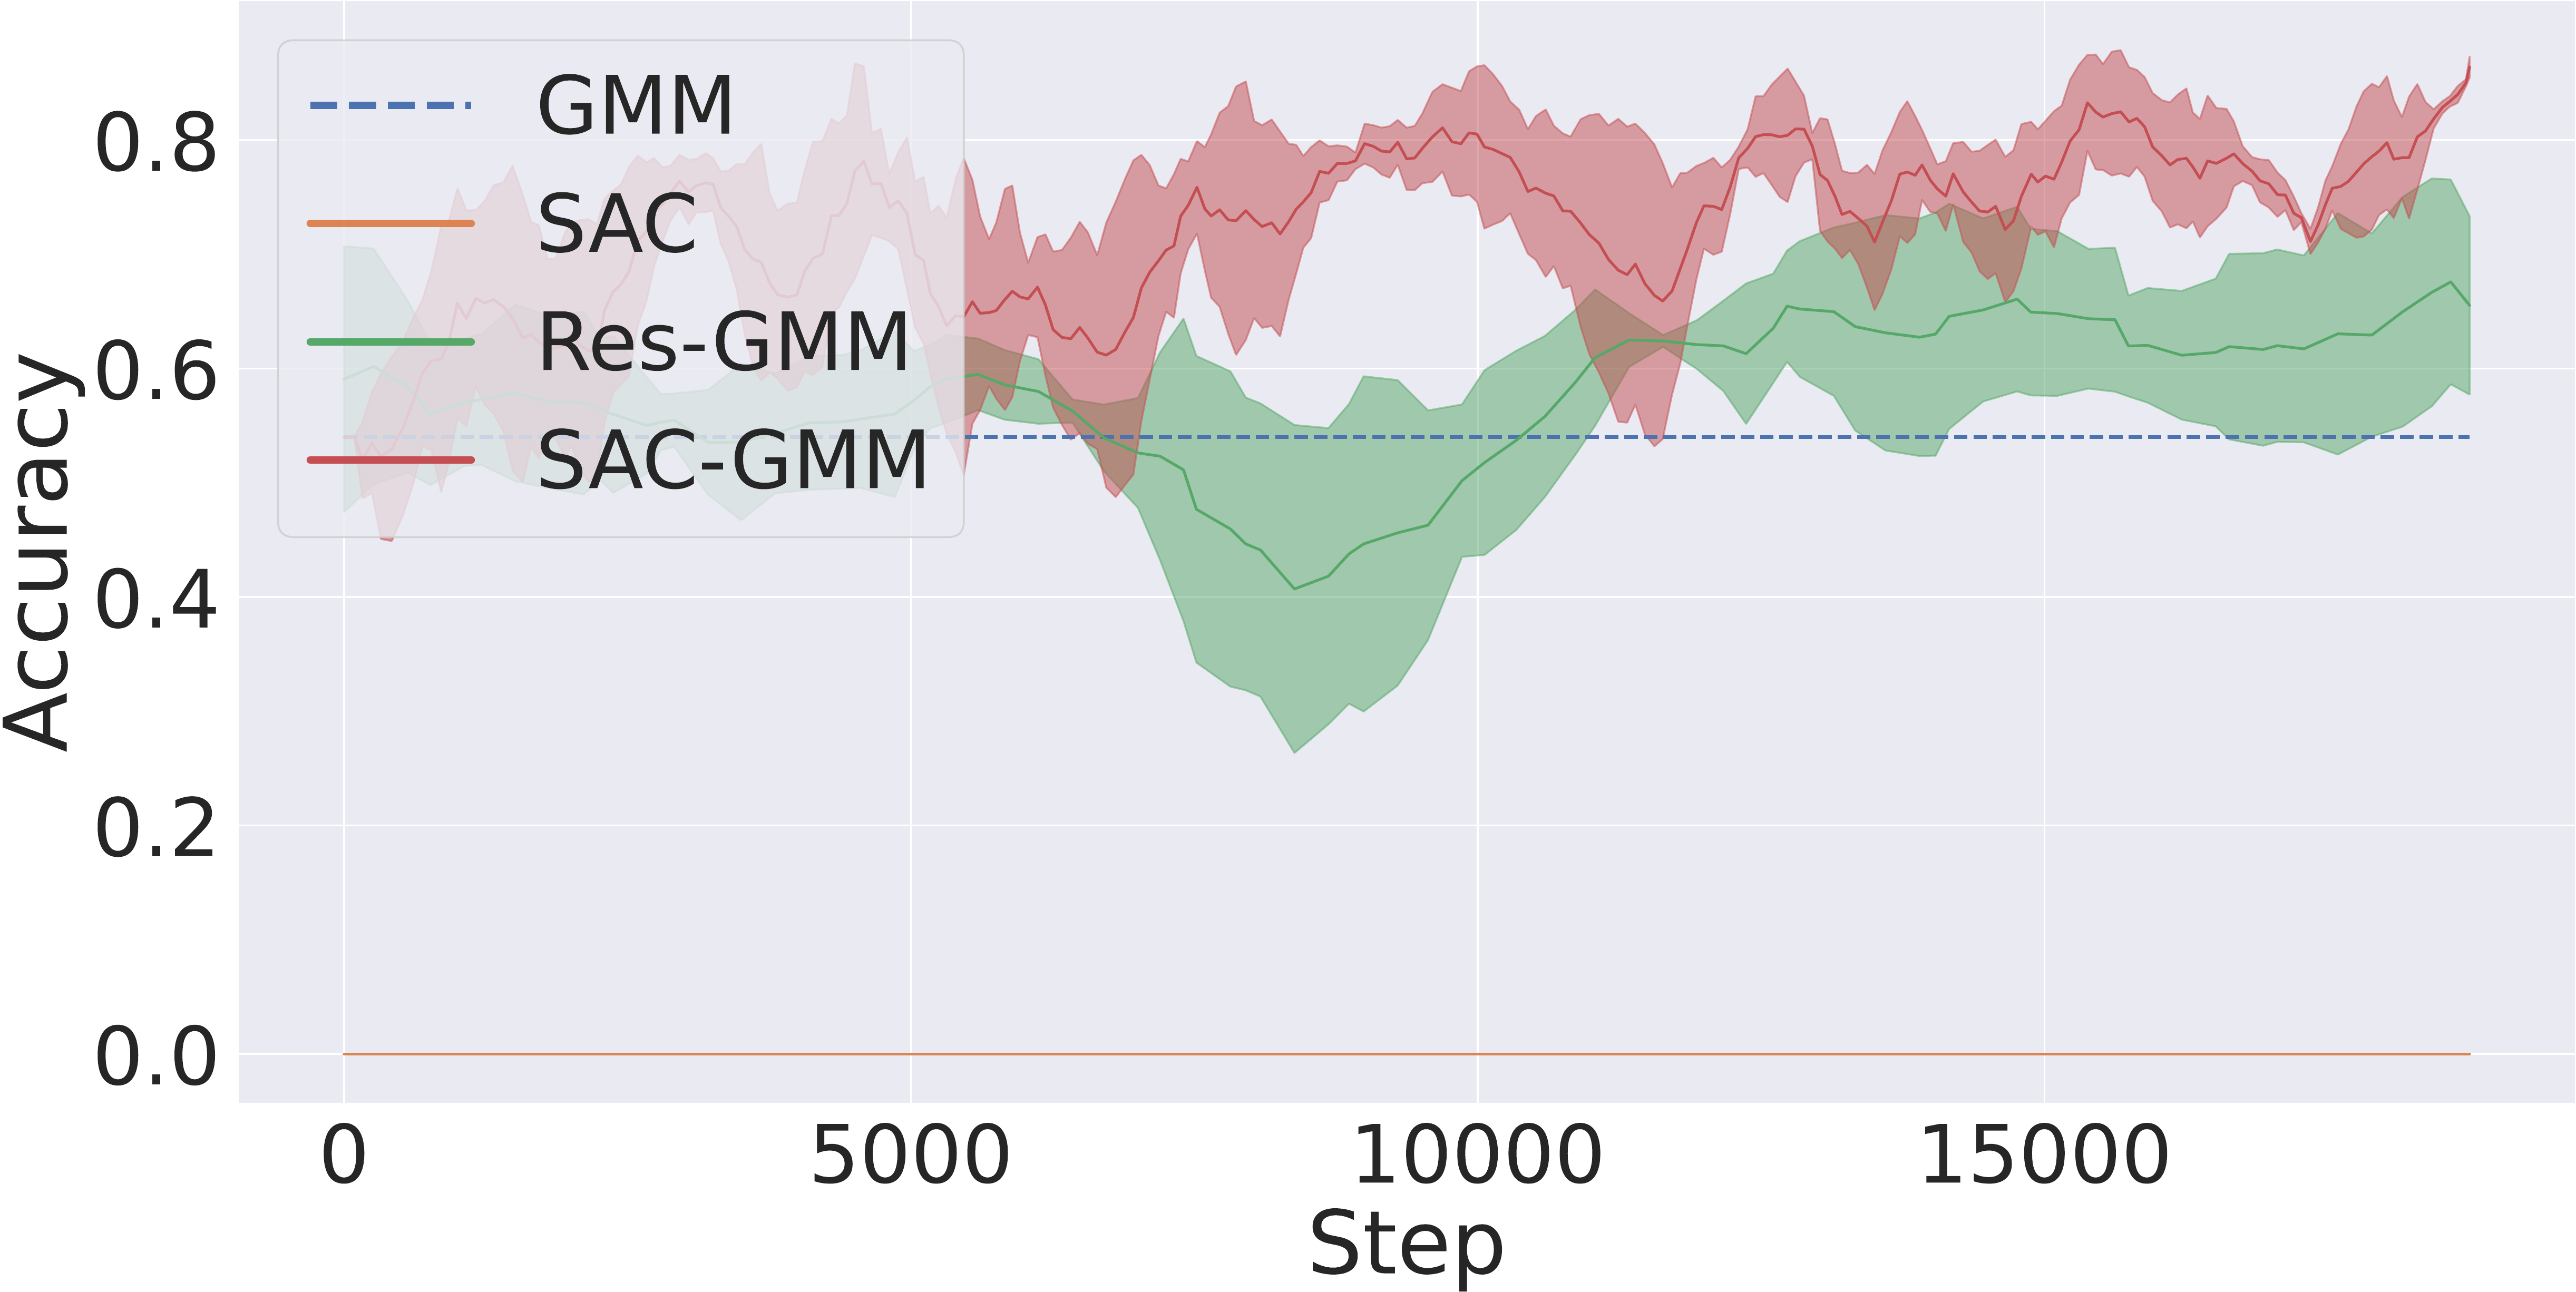}
    \caption{Rewards obtained of the different baselines in the two tasks over their training process.}
    \label{fig:reward_plots}
\end{figure}

\begin{figure}[b]
    \centering
    \includegraphics[height=4.5cm]{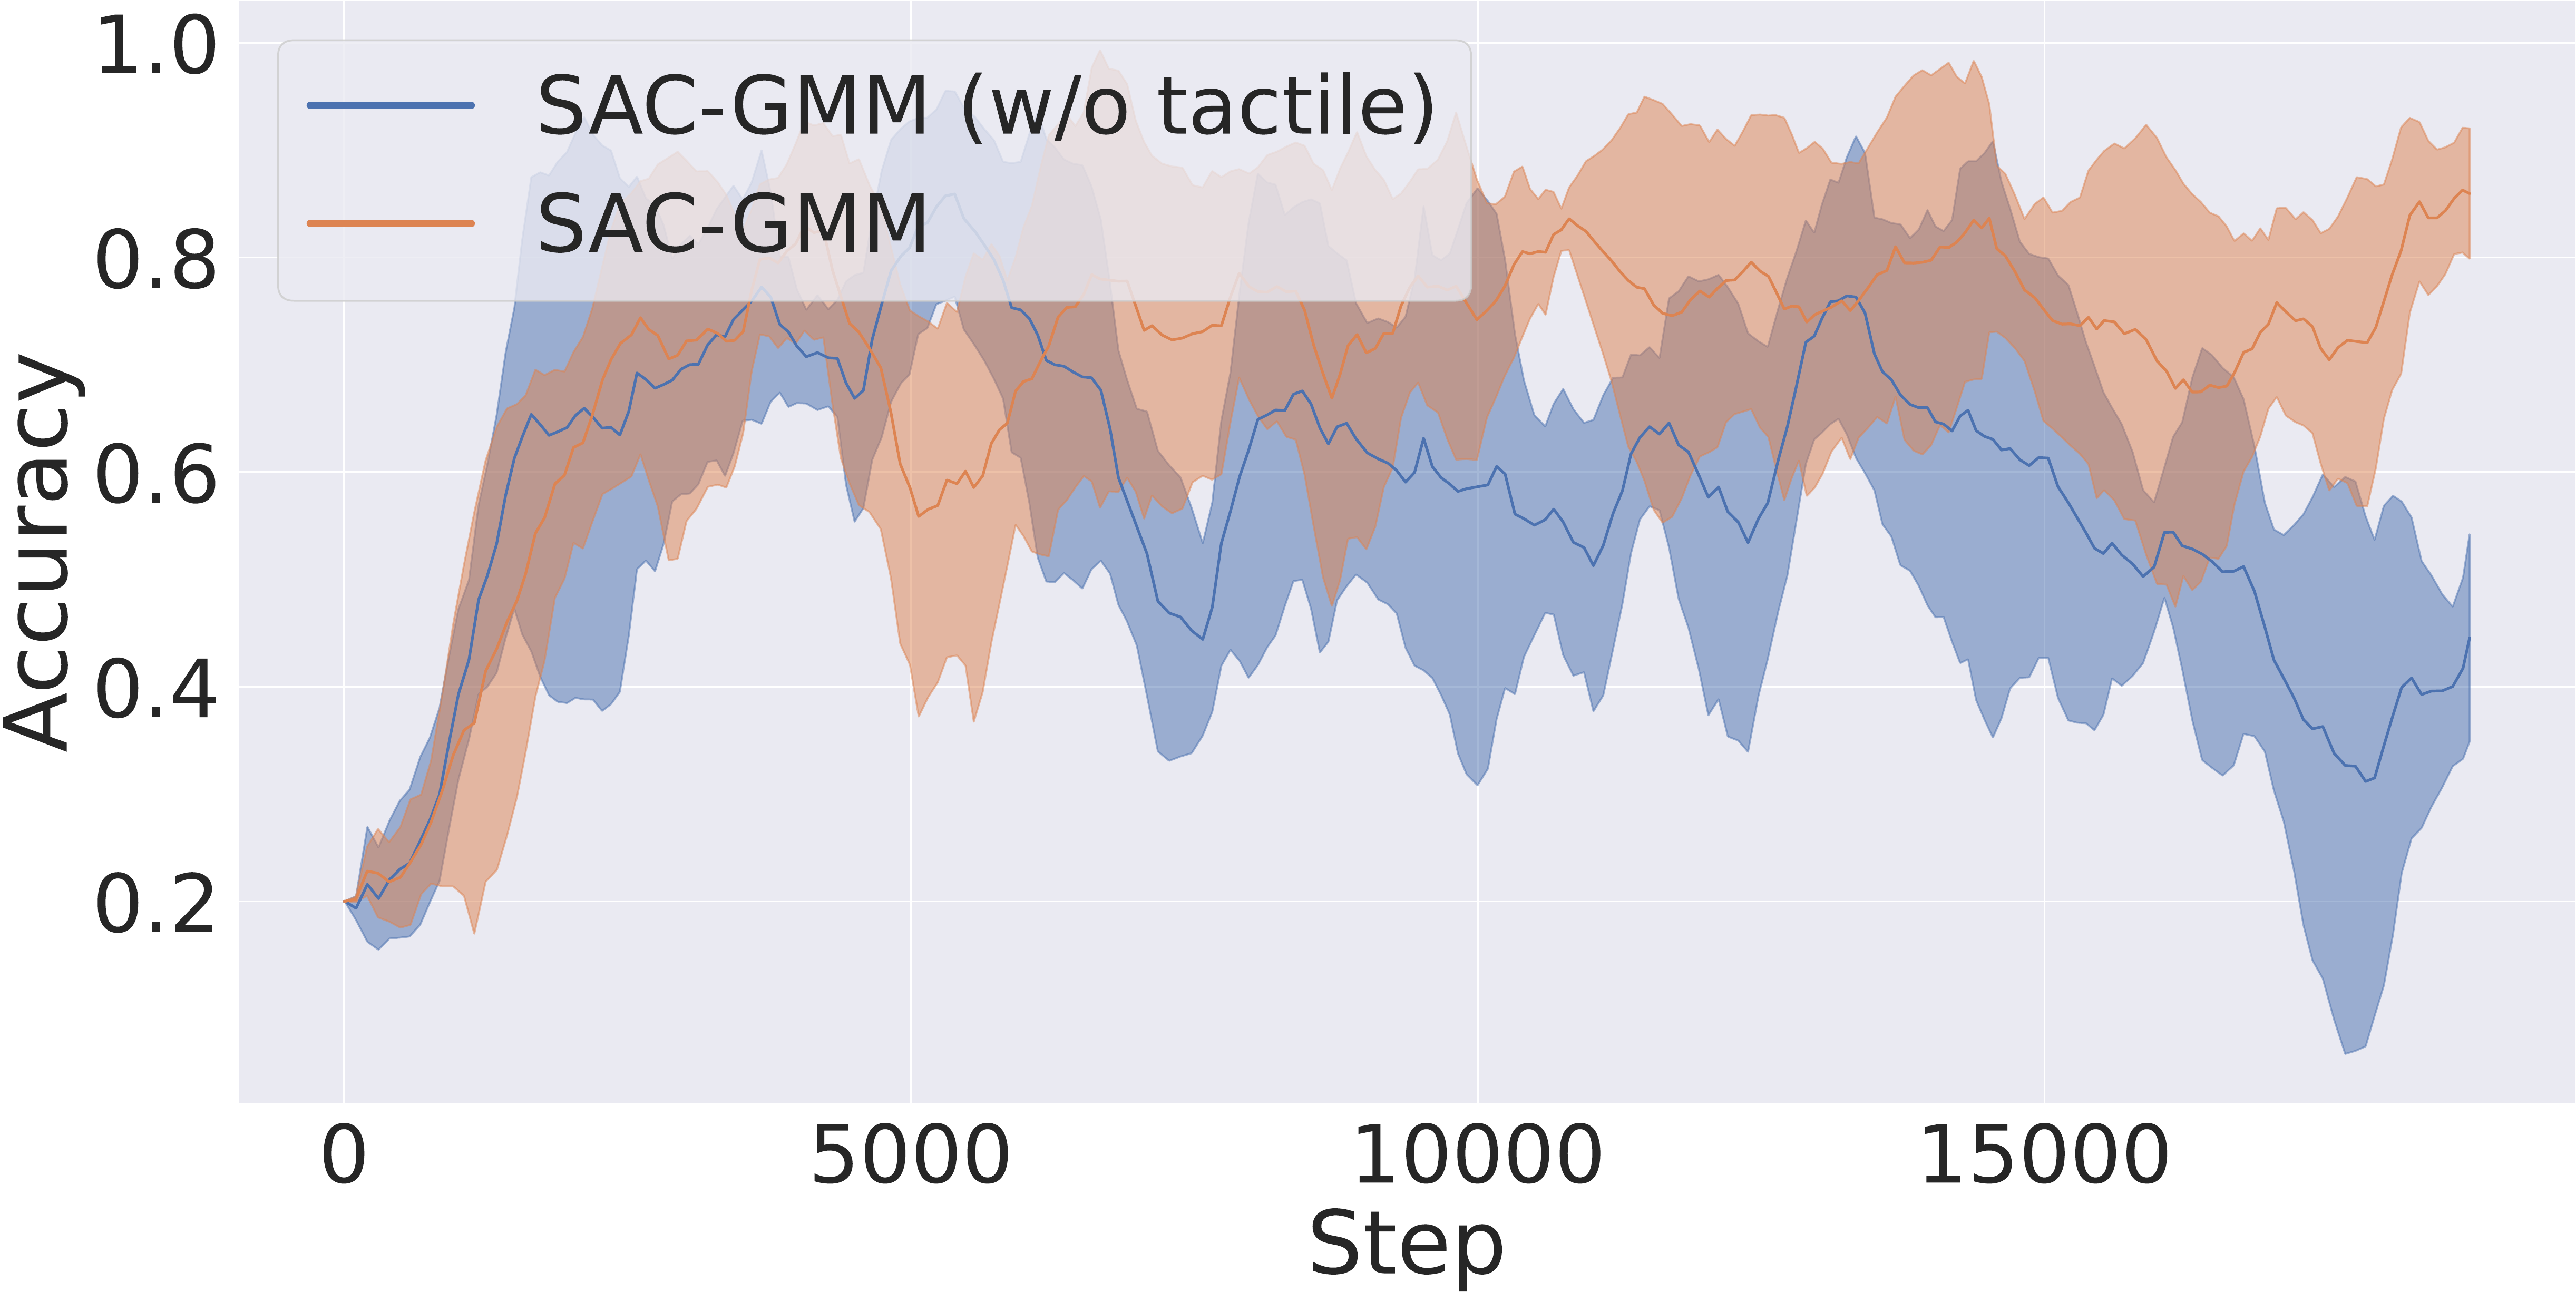}
    \caption{SAC GMM Tactile comparison}
    \label{fig:sac_gmm_tactile_comparison}
\end{figure}

\begin{figure}[b]
    \centering
    \includegraphics[height=4.5cm]{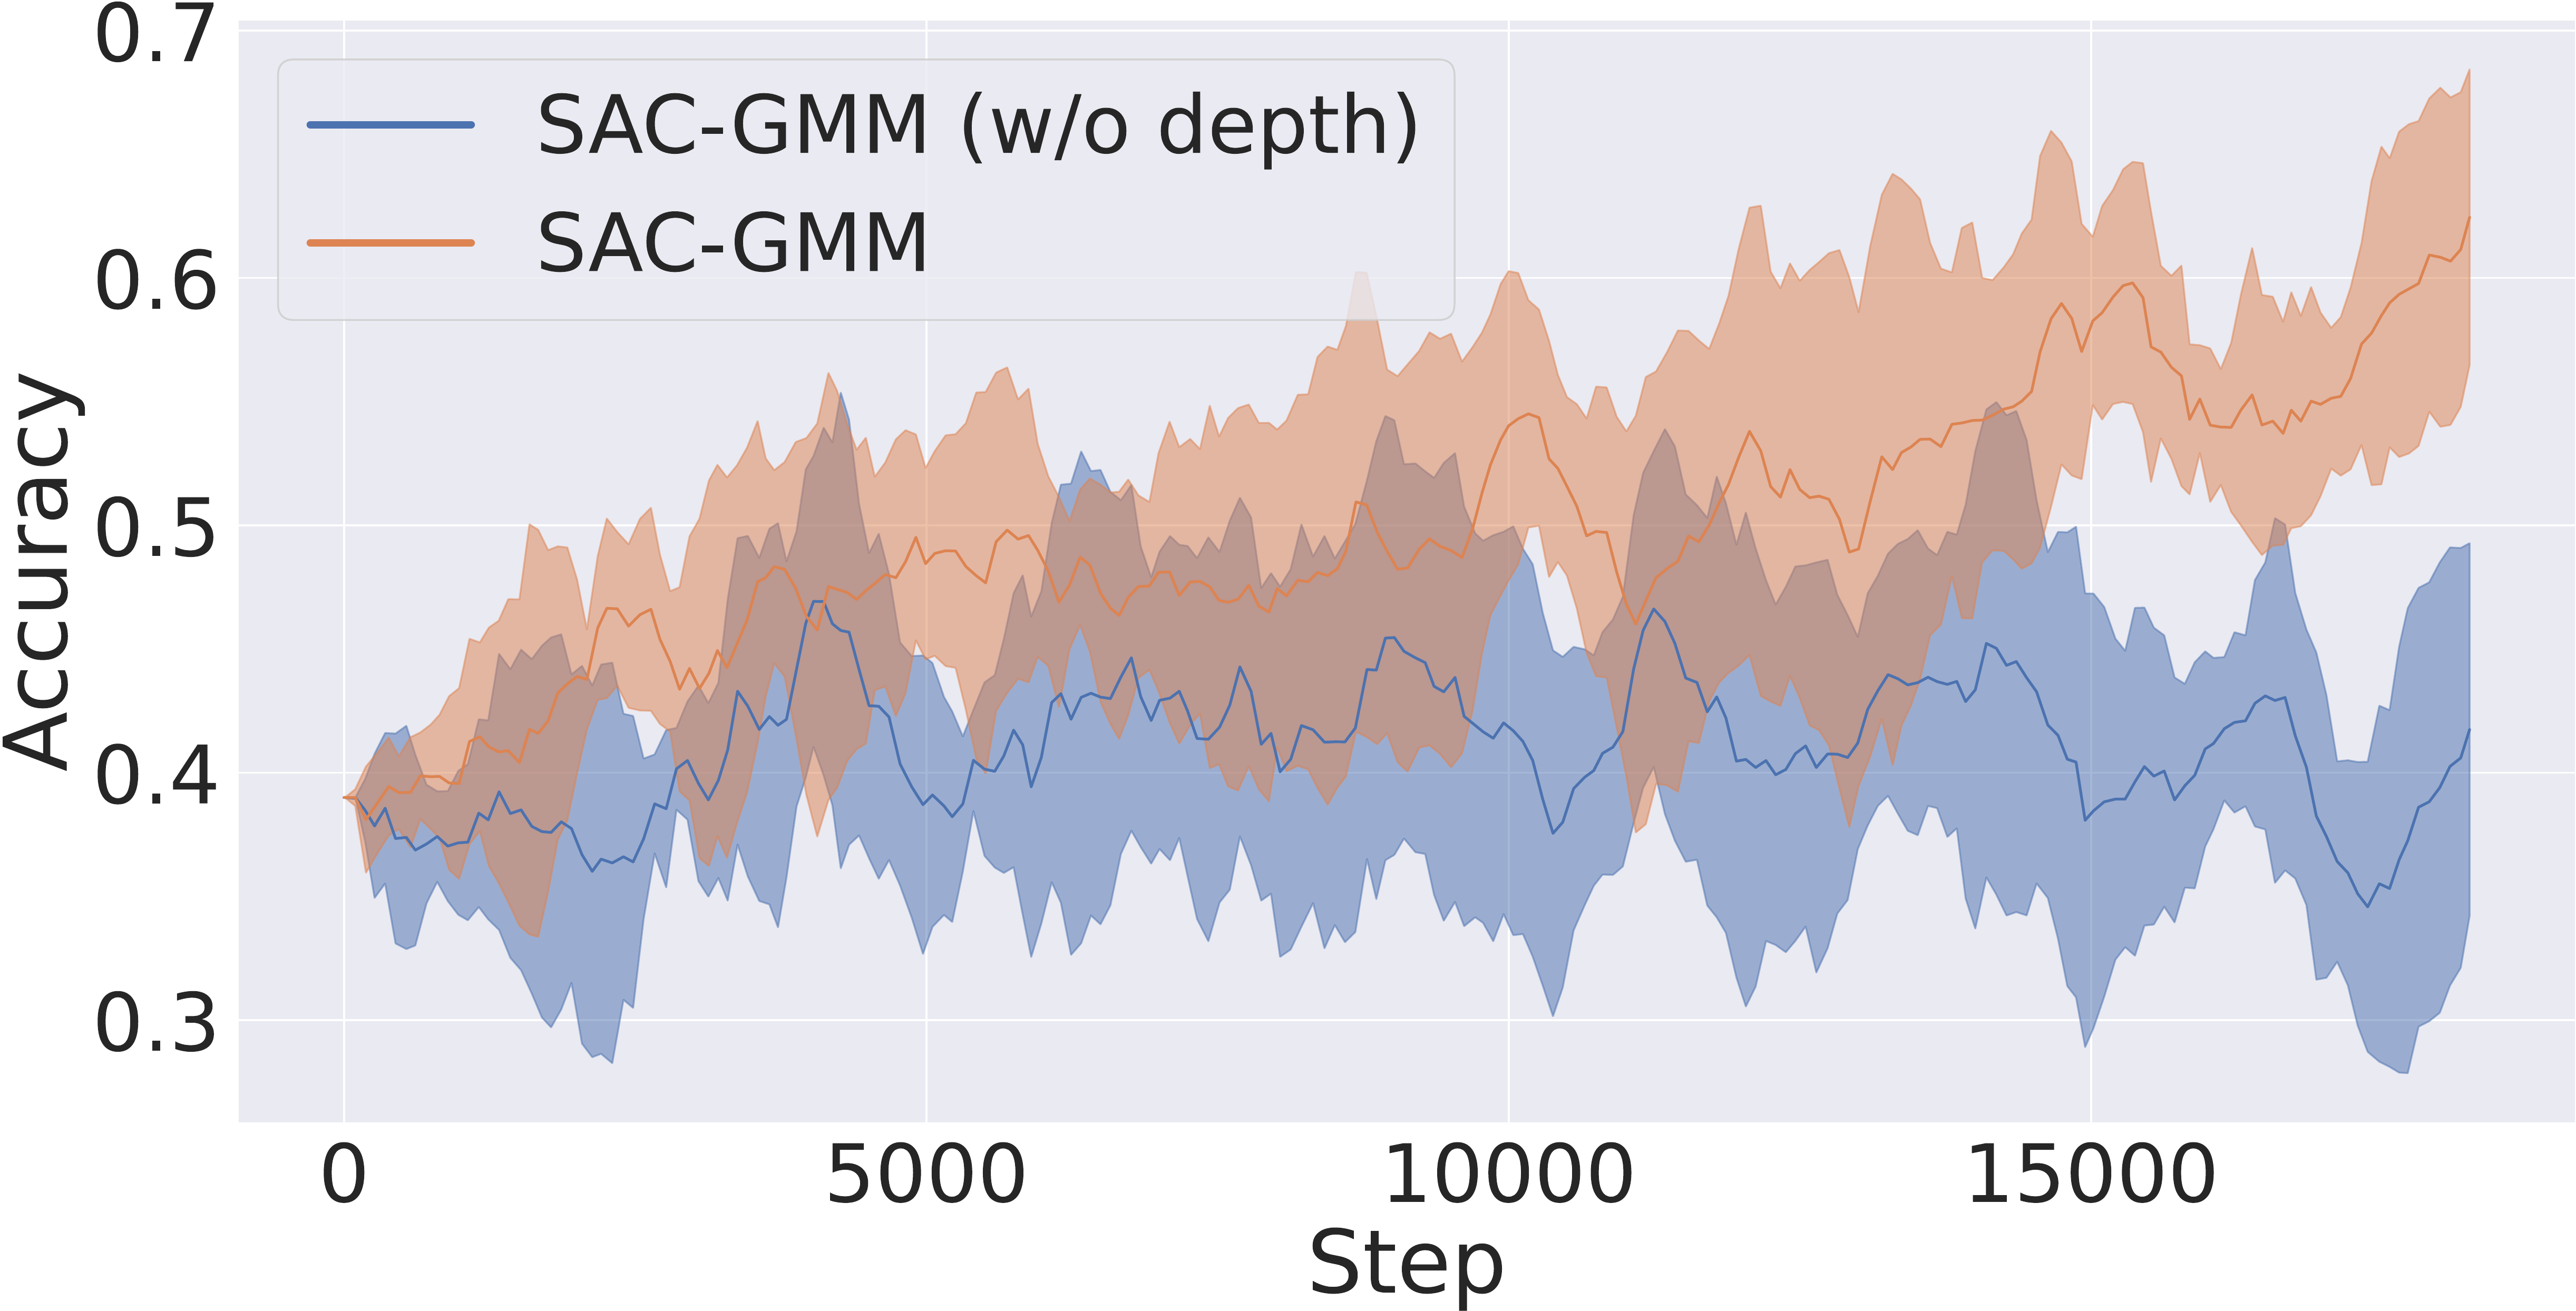}
    \caption{SAC GMM Noise Depth comparison}
    \label{fig:sac_gmm_noise_depth_comparison}
\end{figure}

\begin{figure}[b]
    \centering
    \includegraphics[height=4.5cm]{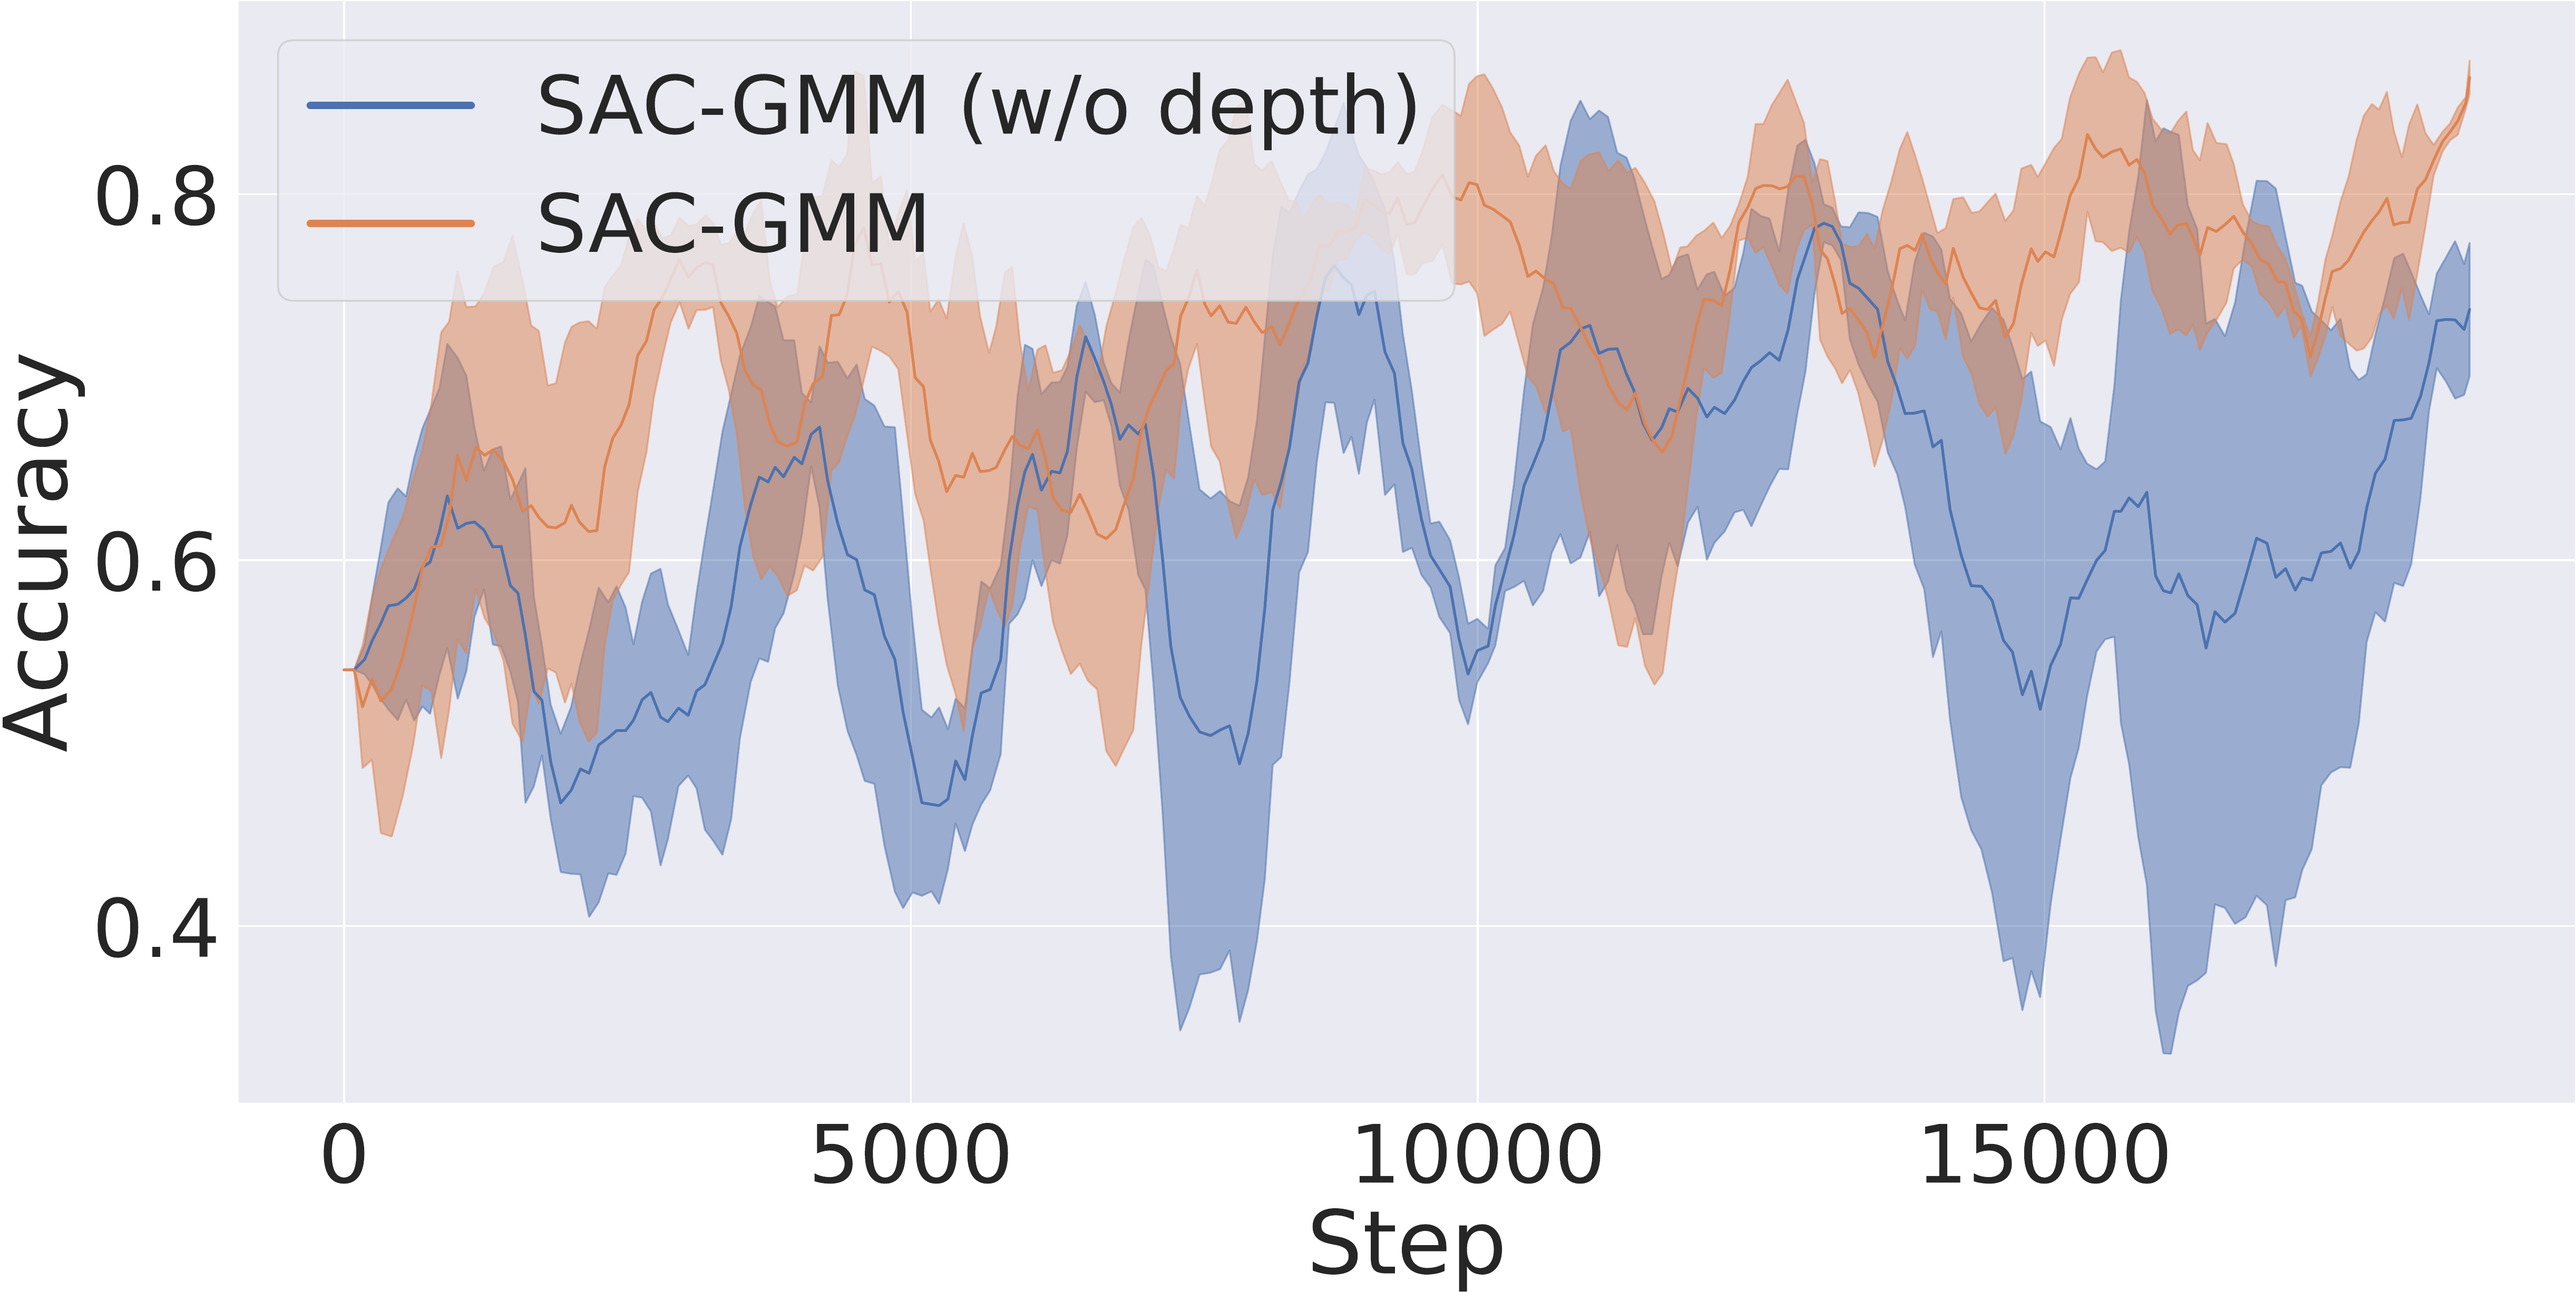}
    \caption{SAC GMM Depth comparison}
    \label{fig:sac_gmm_depth_comparison}
\end{figure}

\subsection{Dynamical System: Gaussian Mixture Model Agent}
Dynamical systems afford an analytical representation of the robot's progression over time, and accordingly, they enable the robot to predict trajectories, be robust in the face of perturbations, and guaranty convergence to a goal. 
%An autonomous dynamical system is a dynamical system that does not explicitly depend on time and employs a first-order ordinary differential equation to map the robot pose to its velocity. Hence, w
We formulate a robot skill as a control law driven by an autonomous dynamical system, defined by the robot pose $\pose$:
\begin{equation}\label{eq:ODE}
    \dpose = f_{\gmmparam}(\pose) + \boldsymbol{\epsilon},
\end{equation}
where $f_{\gmmparam}$ is the robot skill model, a parametric, non-linear, steady, and continuously differentiable function, and $\boldsymbol{\epsilon}$ is a zero-mean additive Gaussian noise. From a machine learning perspective, learning the noise-free estimate of $f$ from data is a regression problem and can be addressed by a mixture of Gaussians. Given a set of reference demonstrations $\demos$ for a robot skill, we parametrize \eqnref{eq:ODE} through Gaussian Mixture Regression (GMR)~\cite{calinon2010learning}. We first estimate the joint probability density of the robot pose and its corresponding first-order derivative by a Gaussian mixture. A Gaussian Mixture Model (GMM) is a linear superposition of multivariate Gaussian distributions, aiming to capture a model for the density of the non-linear robot skill exhibited in demonstrations. A GMM with $K$ Gaussian components represents the joint probability of the robot pose $\pose$ and the corresponding velocity $\dpose$ by
\begin{equation}\label{eq:gmm}
    \mathcal{P}(\pose, \dpose) = \sum_{k=1}^{K} \mathcal{P}(k) \mathcal{P}(\pose, \dpose\given k),
\end{equation}
where $\mathcal{P}(k)$ is a prior and $\mathcal{P}(\pose, \dpose \given k)$ is the joint probability density corresponding to the $k$-th Gaussian. Therefore, we parametrize the robot skill model $f$ by $\gmmparam=\{\prior_k,\mean_k, \cov_k \}_{k = 1}^K$, where $\prior_k$ is the prior (or mixing weight), $\mean_k$ the mean and $\cov_k$ the covariance of the $k$-th Gaussian function. The means and covariances are defined by:
\begin{equation}

\mean^k = 
\begin{pmatrix}
\mean_{\pose}^k \\
\mean_{\dpose}^k 
\end{pmatrix}
\quad\text{and}\quad
\cov^k = 
\begin{pmatrix}
\cov^k_{\pose} & \cov^k_{\pose \dpose}\\
\cov^k_{\dpose\pose} & \cov^k_{\dpose}
\end{pmatrix}.
\end{equation}

Maximum-likelihood estimation of the mixture parameters can be carried out iteratively with different optimization techniques such as Expectation-Maximization (EM) algorithms~\cite{dempster1977maximum,coates2008learning} or more sophisticated approaches that additionally ensure stability and convergence of the dynamical system as~\cite{khansari2011learning} or~\cite{figueroa2018physically} which we use in this work.
By using this estimated joint probability density function, we employ Gaussian mixture regression (GMR) to retrieve $\dpose$ given $\pose$ as the conditional distribution $\mathcal{P}(\dpose \given \pose)$:
\begin{align}
\predmean_{\dpose} &= \sum_{k=1}^{K} h_k(\pose) \left(\mean^k_{\dpose} +
	\cov^k_{\dpose\pose}\left(\cov^k_{\pose}\right)^{-1} 
	\left(\pose-\mean^k_{\pose}\right)\right),
\\
\predcov_{\dpose} &= \sum_{k=1}^{K} h^2_k(\pose) 
				\left(\cov^k_{\dpose} -
				\cov^k_{\dpose \pose} \left(\cov^k_{ \pose}\right)^{-1} \cov^k_{\pose\dpose}\right),
\end{align}
where the weights $h_k(\pose)$ correspond to
\begin{equation}
h_k(\pose) = \frac{\mathcal{P}(k)\mathcal{P}(\pose\given k)}{\sum_{k=1}^{K} \mathcal{P}(k) \mathcal{P}(\pose \given k)}
\end{equation}
and $\predmean_{\dpose}$ and $\predcov_{\dpose}$ are the estimated parameters of $\mathcal{P}(\dpose \given \pose)$.

Our skill model can now reproduce the demonstrated skill by estimating the next velocity at the current robot pose. Since $\hat{f}(\pose) = \predmean$ we get: 
\begin{equation}
\dot{\pose} = \sum_{k=1}^{K} h_k(\pose)
\left(\mean^k_{\dpose} +
	\cov^k_{\dpose\pose}\left(\cov^k_{\pose}\right)^{-1} 
	\left(\pose-\mean^k_{\pose}\right)\right).
\end{equation}

We can generate a trajectory for the robot skill by updating the pose $\pose$ with the generated velocity $\dpose$ scaled by a time step and proceeding iteratively.
